# Supplementary material for: Machine learning force fields based on local parametrization of dispersion interactions: Application to the phase diagram of C$_{60}$
Source: arXiv:2105.02525 ancillary file (2021-08-10)
Supplement: Supplementary file 1 [file supplement.pdf]

# Supplemental Information:
# Machine learning force fields based on local parametrization of dispersion interactions: Application to the phase diagram of $C_{60}$

Heikki Muhli,[1] Xi Chen,[1,*] Albert P. Bartók,[2] Patricia Hernández-León,[3]
Gábor Csányi,[4] Tapio Ala-Nissila,[1,5] and Miguel A. Caro[3,†]

[1]*Department of Applied Physics, Aalto University, 02150, Espoo, Finland*
[2]*Department of Physics and Warwick Centre for Predictive Modelling, School of Engineering, University of Warwick, Coventry CV4 7AL, United Kingdom*
[3]*Department of Electrical Engineering and Automation, Aalto University, 02150, Espoo, Finland*
[4]*Engineering Laboratory, University of Cambridge, Cambridge CB2 1PZ, United Kingdom*
[5]*Interdisciplinary Centre for Mathematical Modelling and Department of Mathematical Sciences, Loughborough University, Loughborough, Leicestershire LE11 3TU, United Kingdom*

(Dated: July 14, 2021)

## I. MODIFIED CUTOFF FUNCTION

We have implemented a cutoff function for the Tkatchenko-Scheffler dispersion interaction to make the derivatives (that is, the dispersion forces) smooth and continuous at the vdW cutoff. In addition, we noticed that as the interatomic distance $r_{ij}$ gets close to zero, the damping function of the original method becomes constant, namely $f_{\text{damp}}(r = 0) = \exp(-d)$, while the $1/r^6$ grows indefinitely. The problem is illustrated in Fig. 1. This is why we also decided to include a cutoff for smaller distances. The cutoff function that we use for both cutoffs is polynomial for computational reasons; evaluating a cosine or exponential cutoff function would be more expensive and the damping function has to be evaluated for each atom and their neighbors within the vdW cutoff radius. It can be seen that as the interatomic distance approaches zero, our implementation also approaches zero smoothly while the implementation without the cutoff function blows up. At the cutoff the original implementation abruptly cuts to zero while our model smoothly approaches zero in the buffer region, preserving the continuity of the derivatives.

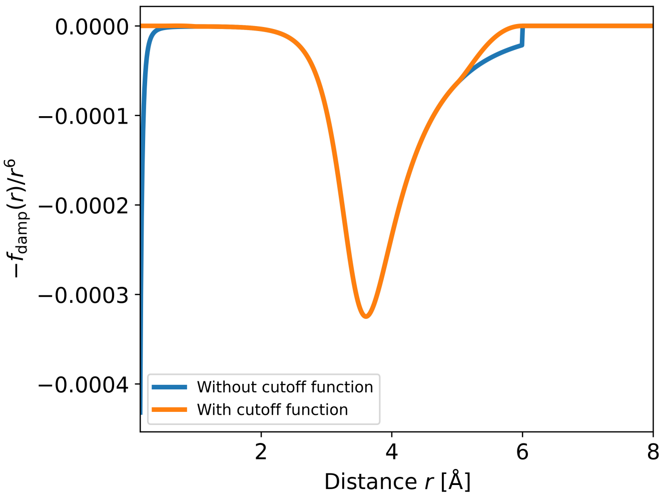


FIG. 1. $-f_{\text{damp}}(r)/r^6$ and $-f_{\text{damp}}(r)f_{\text{cut}}(r)/r^6$ plotted as a function of $r$, the interatomic distance of a carbon dimer. The approaching singularity at $r \to 0$ can be seen with small values of $r$. Here we have used fixed Hirshfeld volumes for the carbon atoms of the dimer to illustrate the problem. The cutoff radius is chosen to be rather short for vdW interactions (6.0 Å) to better illustrate the discontinuity at the cutoff with the original approach. We have chosen a buffer region of 1.0 Å where the interaction smoothly switches to zero.

## II. FITTING THE EFFECTIVE HIRSHFELD VOLUMES

We use the methodology we described for Gaussian approximation potentials to predict new Hirshfeld volumes from DFT data calculated with VASP [1, 2] at the PBE [3] level with TS [4] dispersion correction. For our purposes we denote the matrix containing the descriptors of the whole training set as $\mathbf{Q} \in \mathbb{R}^{N \times N_{\text{SOAP}}}$ and the matrix containing only the sparsified set as $\mathbf{Q}_S \in \mathbb{R}^{N_S \times N_{\text{SOAP}}}$. The sparse set is a subset of representative atomic environments (or pairs and triplets in case of two-body and three-body descriptors) of the training set [5, 6] which is a subset of atomic structures of the whole data set. The remaining data set left out of the training set is the test set that is used to validate the model. We choose the training set and the sparse set randomly but furthest point sampling can be used to slightly improve the representation of the whole data set. In this case the distance between the points in the set can be calculated, for example, by using the kernel distance:

$$D(i, \{s\}) = \sum_{s \in S} \sqrt{1 - k(i, s)}. \quad (1)$$

Here $s \in S$ are points already in the sparse set and the next point is found by maximizing the distance (1). The first point can be chosen by maximizing the equation for the entire training set such that the most distant point in the entire training set is the first point in the sparse set. This procedure gives the best representation of the whole training set for sufficiently large sparse set but the change in the error is usually negligible compared to random sampling.

* xi.6.chen@aalto.fi
† mcaroba@gmail.com

After exponentiation with $\zeta$ and sparsification, the following set of equations defines the regularized and sparsified ML model [5]:

$$\mathbf{C}_{SS} = (\mathbf{Q}_S\mathbf{Q}_S^T)^{\odot\zeta} + \sigma_{\text{jitter}}\mathbf{I}_{N_S}, \quad \mathbf{C}_{ST} = (\mathbf{Q}_S\mathbf{Q}^T)^{\odot\zeta},$$
$$\mathbf{C}_{TS} = \mathbf{C}_{ST}^T \quad \mathbf{\Lambda}_{TT} = \sigma_n^2\mathbf{I}_N,$$
$$\boldsymbol{\alpha} = (\mathbf{C}_{SS} + \mathbf{C}_{ST}\mathbf{\Lambda}_{TT}^{-1}\mathbf{C}_{TS})^{-1}\mathbf{C}_{ST}\mathbf{\Lambda}_{TT}^{-1}\boldsymbol{\nu},$$
$$\nu_i = (\mathbf{q}_i\mathbf{Q}_S^T)^{\odot\zeta}\boldsymbol{\alpha}. \quad (2)$$

Here $\mathbf{I}_N \in \mathbb{R}^{N\times N}$ is the identity matrix, the vector $\boldsymbol{\nu}$ contains the Hirshfeld volumes calculated using DFT (usually shifted by approximately the mean of the volumes to improve the fit) and $\sigma_n^2$ can be tuned to reduce overfitting. The small positive value $\sigma_{\text{jitter}}$ (usually approximately 6-9 orders of magnitude smaller than the diagonal elements [5]) is added to the diagonal of $\mathbf{C}_{SS}$ such that the sparsified kernel matrix preserves its positive-definiteness and the model is more stable. The Hadamard operation is denoted by "$\odot$" and means element-wise exponentiation in the equations above. The last equation can be equivalently written as:

$$\nu_i = \sum_{s\in S}\alpha_s k(i,s)^\zeta. \quad (3)$$

## III. DETAILS OF DISPERSION FORCE CALCULATION

The analytical dispersion forces are given as the negative gradient of the dispersion energy of the structure:

$$f_k^\alpha = -\frac{\partial E_{\text{TS}}}{\partial r_k^\alpha}. \quad (4)$$

Here $r_k^\alpha$ is the Cartesian component of the position of atom $k$ in the molecule or the unit cell. Using the Eq. (1) in the main manuscript for $E_{\text{TS}}$ and the product rule of derivatives we get

$$f_k^\alpha = \frac{1}{2}\sum_i\sum_{j\neq i}\frac{\partial C_{6,ij}}{\partial r_k^\alpha}\frac{f_{\text{damp}}(r_{ij})f_{\text{cut}}(r_{ij})}{r_{ij}^6} + \frac{\partial}{\partial r_k^\alpha}\left(\frac{1}{r_{ij}^6}\right)C_{6,ij}f_{\text{damp}}(r_{ij})f_{\text{cut}}(r_{ij}) + \frac{\partial f_{\text{damp}}}{\partial r_k^\alpha}\frac{C_{6,ij}f_{\text{cut}}(r_{ij})}{r_{ij}^6} + \frac{\partial f_{\text{cut}}}{\partial r_k^\alpha}\frac{C_{6,ij}f_{\text{damp}}(r_{ij})}{r_{ij}^6}. \quad (5)$$

The dipole-dipole dispersion coefficient can be written explicitly as a function of Hirshfeld volumes of atoms $A$ and $B$ and after simplifying we get

$$C_{6,ij} = \frac{2\nu_i\nu_j C_{6,ii}^{\text{free}}C_{6,jj}^{\text{free}}}{\frac{\alpha_{j,0}^{\text{free}}}{\alpha_{i,0}^{\text{free}}}C_{6,ii}^{\text{free}} + \frac{\alpha_{i,0}^{\text{free}}}{\alpha_{j,0}^{\text{free}}}C_{6,jj}^{\text{free}}} = \nu_i\nu_j C_{6,ij}^{\text{free}}, \quad (6)$$

where in the last equality we have defined $C_{6,ij}^{\text{free}}$ as the dipole-dipole dispersion coefficient with corresponding free-atom values. The derivative of the coefficient is given by

$$\frac{\partial C_{6,ij}}{\partial r_k^\alpha} = \left(\frac{\partial\nu_i}{\partial r_k^\alpha}\nu_j + \nu_i\frac{\partial\nu_j}{\partial r_k^\alpha}\right)C_{6,ij}^{\text{free}}. \quad (7)$$

The interatomic distance is defined as

$$r_{ij} = |\mathbf{r}_j - \mathbf{r}_i| = \sqrt{\sum_\beta(r_j^\beta - r_i^\beta)^2}, \quad (8)$$

where $\mathbf{r}_i$ and $\mathbf{r}_j$ are the position vectors of atoms $i$ and $j$, respectively and $\beta$ denotes the Cartesian components. The second derivative in (5) is then given by

$$\frac{\partial}{\partial r_k^\alpha}\left(\frac{1}{r_{ij}^6}\right) = -\frac{6}{r_{ij}^7}\left(\frac{1}{2\sqrt{\sum_\beta(r_j^\beta - r_i^\beta)^2}}\right)2(r_j^\alpha - r_i^\alpha)(\delta_{jk} - \delta_{ik}) = -\frac{6}{r_{ij}^8}(r_j^\alpha - r_i^\alpha)(\delta_{jk} - \delta_{ik}), \quad (9)$$

where $\delta_{jk}$ is the Kronecker delta that has the property $\delta_{jk} = 1$ if $j = k$ and $\delta_{jk} = 0$ otherwise.

The derivative of the damping function is given by

$$\frac{\partial f_{\text{damp}}}{\partial r_k^\alpha} = -f_{\text{damp}}(r_{ij})^2\exp\left(-d\left(\frac{r_{ij}}{s_R r_{ij}^{\text{vdW}}} - 1\right)\right) \times\left(-\frac{d}{s_R}\frac{\partial}{\partial r_k^\alpha}\left(\frac{r_{ij}}{r_{ij}^{\text{vdW}}}\right)\right). \quad (10)$$

The last derivative is calculated using the product rule

$$\frac{\partial}{\partial r_k^\alpha}\left(\frac{r_{ij}}{r_{ij}^{\text{vdW}}}\right) = \frac{\partial r_{ij}}{\partial r_k^\alpha}\frac{1}{r_{ij}^{\text{vdW}}} + r_{ij}\frac{\partial}{\partial r_k^\alpha}\left(\frac{1}{r_{ij}^{\text{vdW}}}\right) = \frac{(r_j^\alpha - r_i^\alpha)(\delta_{jk} - \delta_{ik})}{r_{ij}r_{ij}^{\text{vdW}}} - \frac{r_{ij}}{(r_{ij}^{\text{vdW}})^2}\frac{\partial r_{ij}^{\text{vdW}}}{\partial r_k^\alpha}. \quad (11)$$

The derivative of the effective van der Waals radius in the last term is obtained by using the expressions for $r_i^{\text{vdW}}$ and $r_{ij}^{\text{vdW}}$ in Eq. (1) of the main manuscript:

$$\frac{\partial r_{ij}^{\text{vdW}}}{\partial r_k^\alpha} = \frac{1}{3\nu_i^{2/3}}\frac{\partial\nu_i}{\partial r_k^\alpha}r_{i,\text{free}}^{\text{vdW}} + \frac{1}{3\nu_j^{2/3}}\frac{\partial\nu_j}{\partial r_k^\alpha}r_{j,\text{free}}^{\text{vdW}} \quad (12)$$

Plugging all of this into Eq. (5) we get:

$$f_k^\alpha = \frac{1}{2}\sum_i \sum_{j\neq i}\left(\frac{\partial v_i}{\partial r_k^\alpha} v_j + v_i \frac{\partial v_j}{\partial r_k^\alpha}\right) C_{6,ij}^{\text{free}} \frac{f_{\text{damp}}(r_{ij}) f_{\text{cut}}(r_{ij})}{r_{ij}^6} + \left(-\frac{6}{r_{ij}^8}(r_j^\alpha - r_i^\alpha)(\delta_{jk} - \delta_{ik})\right) C_{6,ij} f_{\text{damp}}(r_{ij}) f_{\text{cut}}(r_{ij})$$
$$+ \frac{d}{s_R} f_{\text{damp}}(r_{ij})^2 \exp\left(-d\left(\frac{r_{ij}}{s_R r_{ij}^{\text{vdW}}} - 1\right)\right)\left[\frac{(r_j^\alpha - r_i^\alpha)(\delta_{jk} - \delta_{ik})}{r_{ij} r_{ij}^{\text{vdW}}} - \frac{r_{ij}}{(r_{ij}^{\text{vdW}})^2}\left(\frac{1}{3v_i^{2/3}} \frac{\partial v_i}{\partial r_k^\alpha} r_{i,\text{free}}^{\text{vdW}} + \frac{1}{3v_j^{2/3}} \frac{\partial v_j}{\partial r_k^\alpha} R_{j,\text{free}}^{\text{vdW}}\right)\right] \frac{C_{6,ij} f_{\text{cut}}(r_{ij})}{r_{ij}^6}$$
$$+ \frac{C_{6,ij} f_{\text{damp}}(r_{ij})}{r_{ij}^6} \frac{\partial f_{\text{cut}}}{\partial r_k^\alpha}. \quad (13)$$

It is convenient to separate the terms that depend on the derivatives of the Hirshfeld volumes from the rest that only include pairwise interactions between atoms $i$ and $j$:

$$f_k^\alpha = \frac{1}{2}\sum_i \sum_{j\neq i} \frac{\partial v_i}{\partial r_k^\alpha} v_j C_{6,ij}^{\text{free}} \frac{f_{\text{damp}}(r_{ij}) f_{\text{cut}}(r_{ij})}{r_{ij}^6} - \frac{r_{ij}}{(r_{ij}^{\text{vdW}})^2} \frac{d}{s_R} f_{\text{damp}}(r_{ij})^2 \exp\left(-d\left(\frac{r_{ij}}{s_R r_{ij}^{\text{vdW}}} - 1\right)\right) \frac{C_{6,ij} f_{\text{cut}}(r_{ij})}{r_{ij}^6} \frac{1}{3v_i^{2/3}} \frac{\partial v_i}{\partial r_k^\alpha} r_{i,\text{free}}^{\text{vdW}}$$
$$+ v_i \frac{\partial v_j}{\partial r_k^\alpha} C_{6,ij}^{\text{free}} \frac{f_{\text{damp}}(r_{ij}) f_{\text{cut}}(r_{ij})}{r_{ij}^6} - \frac{r_{ij}}{(r_{ij}^{\text{vdW}})^2} \frac{d}{s_R} f_{\text{damp}}(r_{ij})^2 \exp\left(-d\left(\frac{r_{ij}}{s_R r_{ij}^{\text{vdW}}} - 1\right)\right) \frac{C_{6,ij} f_{\text{cut}}(r_{ij})}{r_{ij}^6} \frac{1}{3v_j^{2/3}} \frac{\partial v_j}{\partial r_k^\alpha} r_{j,\text{free}}^{\text{vdW}}$$
$$+ \frac{C_{6,ij}}{r_{ij}^7} f_{\text{damp}}(r_{ij}) f_{\text{cut}}(r_{ij})(r_j^\alpha - r_i^\alpha)(\delta_{jk} - \delta_{ik})\left[-\frac{6}{r_{ij}} + \frac{d}{s_R r_{ij}^{\text{vdW}}} f_{\text{damp}}(r_{ij}) \exp\left(-d\left(\frac{r_{ij}}{s_R r_{ij}^{\text{vdW}}} - 1\right)\right)\right] + \frac{C_{6,ij} f_{\text{damp}}(r_{ij})}{r_{ij}^6} \frac{\partial f_{\text{cut}}}{\partial r_k^\alpha}. \quad (14)$$

Here the first and second line are essentially double counting the same interactions. The same happens with the third line involving Kronecker deltas: the term $(r_j^\alpha - r_i^\alpha)(\delta_{jk} - \delta_{ik})$ gets double counted and can be replaced with $2(r_j^\alpha - r_i^\alpha)(-\delta_{ik})$. The actual form of the derivative of the cut-off function is given as:

$$\frac{\partial f_{\text{cut}}}{\partial r_k^\alpha} = \begin{cases} -\frac{6}{d_{\text{b,o}}} \frac{(r_j^\alpha - r_i^\alpha)}{r_{ij}} (\delta_{jk} - \delta_{ik})(-r_{\text{b,o}} + r_{\text{b,o}}^2), & \text{if } r_{\text{c,o}} - d_{\text{b,o}} < r_{ij} \leq r_{\text{c,o}} \\ -\frac{6}{d_{\text{b,i}}} \frac{(r_j^\alpha - r_i^\alpha)}{r_{ij}} (\delta_{jk} - \delta_{ik})(r_{\text{b,i}} - r_{\text{b,i}}^2), & \text{if } r_{\text{c,i}} < r_{ij} \leq r_{\text{c,i}} + d_{\text{b,i}} \\ 0, & \text{otherwise,} \end{cases} \quad (15)$$

which also includes the same Kronecker deltas and which can be modified in a similar fashion. Taking all the double counting into account we can simplify the equation further (and get rid of the multiplier $1/2$ in front) arriving in the form we gave in the text:

$$f_k^\alpha = \sum_i \frac{\partial v_i}{\partial r_k^\alpha} \sum_{j\neq i}\left[\frac{C_{6,ij}}{v_i} \frac{f_{\text{damp}}(r_{ij})}{r_{ij}^6} f_{\text{cut}}(r_{ij}) - \frac{r_{ij}}{(r_{ij}^{\text{vdW}})^2} \frac{d}{s_R} f_{\text{damp}}(r_{ij})^2 f_{\text{cut}}(r_{ij}) \exp\left(-d\left(\frac{r_{ij}}{s_R r_{ij}^{\text{vdW}}} - 1\right)\right) \frac{C_{6,ij}}{r_{ij}^6} \frac{1}{3v_i^{2/3}} r_{i,\text{free}}^{\text{vdW}}\right]$$
$$+ \sum_i \delta_{ik} \sum_{j\neq i} \frac{C_{6,ij}}{r_{ij}^7} f_{\text{damp}}(r_{ij}) f_{\text{cut}}(r_{ij})(r_j^\alpha - r_i^\alpha)\left[\frac{6}{r_{ij}} - \frac{d}{s_R r_{ij}^{\text{vdW}}} f_{\text{damp}}(r_{ij}) \exp\left(-d\left(\frac{r_{ij}}{s_R r_{ij}^{\text{vdW}}} - 1\right)\right)\right]$$
$$+ \sum_i \delta_{ik} \sum_{j\neq i} \frac{C_{6,ij}}{r_{ij}^7} f_{\text{damp}}(r_{ij})(r_j^\alpha - r_i^\alpha) D_{ij}, \quad (16)$$

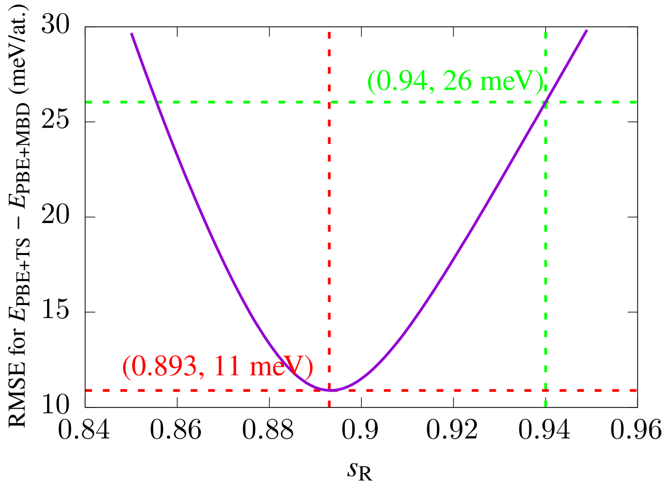


FIG. 2. Optimization of $s_R$ for carbon.

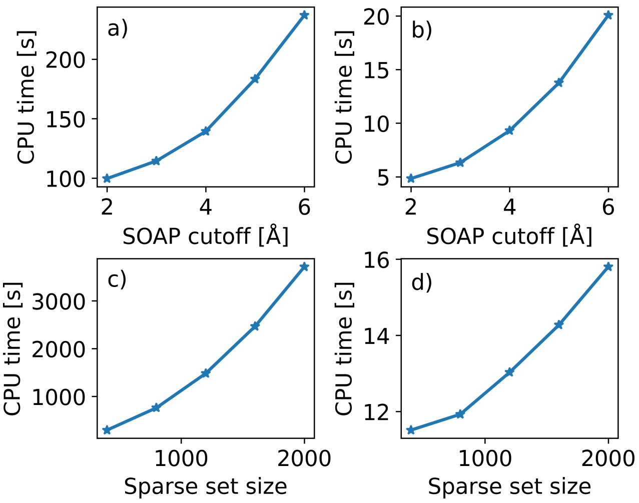


FIG. 3. Timings for fitting and testing the model with different SOAP cutoff radii and sparse set sizes. The fitting and testing were done on a virtual machine, which makes the calculations about twice as slow as without virtualization. a) CPU time as a function of SOAP cutoff for fitting the model with a sparse set size of 200, using the entire training set (4529 carbon structures with an average of approximately 68 carbon atoms per structure). b) Evaluation of the model in figure a) for a-C test set. c) CPU time as a function of the sparse set size for fitting the model with a SOAP cutoff of 4.5 Å using the entire data set. d) Evaluation of the model in figure c) for a-C test set.

with the coefficient $D_{ij}$ that appears due to the derivative of the cut-off function given by the following equation:

$$D_{ij} = \begin{cases} -\frac{6}{d_{\mathrm{b,o}}}(-r_{\mathrm{b,o}} + r_{\mathrm{b,o}}^2), & \text{if } r_{\mathrm{c,o}} - d_{\mathrm{b,o}} < r_{ij} \leq r_{\mathrm{c,o}} \\ -\frac{6}{d_{\mathrm{b,i}}}(r_{\mathrm{b,i}} - r_{\mathrm{b,i}}^2), & \text{if } r_{\mathrm{c,i}} < r_{ij} \leq r_{\mathrm{c,i}} + d_{\mathrm{b,i}} \\ 0, & \text{otherwise.} \end{cases} \quad (17)$$

## IV. OPTIMIZING $s_R$ FOR CARBON

The damping parameter $s_R$ usually used in combination with TS corrections and the PBE functional was originally obtained [4] by minimizing the error in the correlation energy of the S22 dataset [7], using coupled cluster as the reference method. Since this is a very small dataset and it does not contain pure carbon structures, it is reasonable to assume that the optimal damping parameter for carbon might be different. In fact, $s_R$ is strongly functional dependent [8, 9]. To estimate $s_R$ we recomputed the GAP17 database at the PBE+MBD level of theory [10, 11], and minimized the difference between PBE+TS and PBE+MBD as a function of $s_R$. For this purpose, we reconfigured ASE's [12] TS implementation to compute the TS energy for the GAP17 database [13] from $s_R = 0.5$ to $s_R = 1.5$ at 0.1 intervals, and then fitted a kernel-ridge-regression model with Gaussian kernels ($\sigma = 0.25$) and Gaussian-noise regularization ($\sigma_{\mathrm{reg}} = 0.001$) to smooth out the predictions. The RMSE vs $s_R$ data is shown in Fig. 2. As can be seen from the graph, our optimized $s_R = 0.893$ reduces the error of the TS method for carbon structures (assuming PBE+MBD as the "ground truth") by over a factor of 2, from 26 meV/atom for the standard value ($s_R = 0.94$) down to 11 meV/atom.

## V. TIMING FOR FITTING AND EVALUATION

We show how the method scales as the SOAP cutoff radius is increased and as the size of the sparse set grows. The timings can be seen in Fig. 3 for both the calculation of the fitting coefficients using the kernel matrix and evaluation of the model for a set of testing structures once the fitting coefficients have been calculated. It is worth noting that the fitting takes a considerably longer time due to the linear algebra steps but it has to be done only once and the resulting fitting coefficients can be used to evaluate the model for any testing structure.

## VI. EFFECT OF VDW CUTOFF ON THE RESULTS

In this section we present the effects of varying vdW cutoff on the results. In particular, we are interested in testing the convergence of vdW forces with respect to the cutoff. We calculated the analytical VASP and GAP forces with cutoff radii of 5 Å, 10 Å and 20 Å and compared them to the cutoff of 50 Å that we used in the main manuscript for the force benchmarks. This is done to justify the choice of 20 Å cutoff in the MD simulations for $C_{60}$ in the main manuscript. The recalculated dispersion forces along with their RMSE, compared to the 50 Å forces, can be seen in Fig. 4. One can see that the effect of reducing the cutoff from 50 Å to 20 Å is small for the GAP dispersion force calculation, as the RMSE is at least an order of magnitude smaller than when the analytical forces are compared to the finite difference forces calculated with VASP. One should again note that the analytical VASP forces do not include the gradients of the effective Hirshfeld volumes, while the GAP forces do, which gives a partial explanation for the smaller errors in VASP forces. The other reason is the buffer region of the implemented cutoff function for GAP forces that

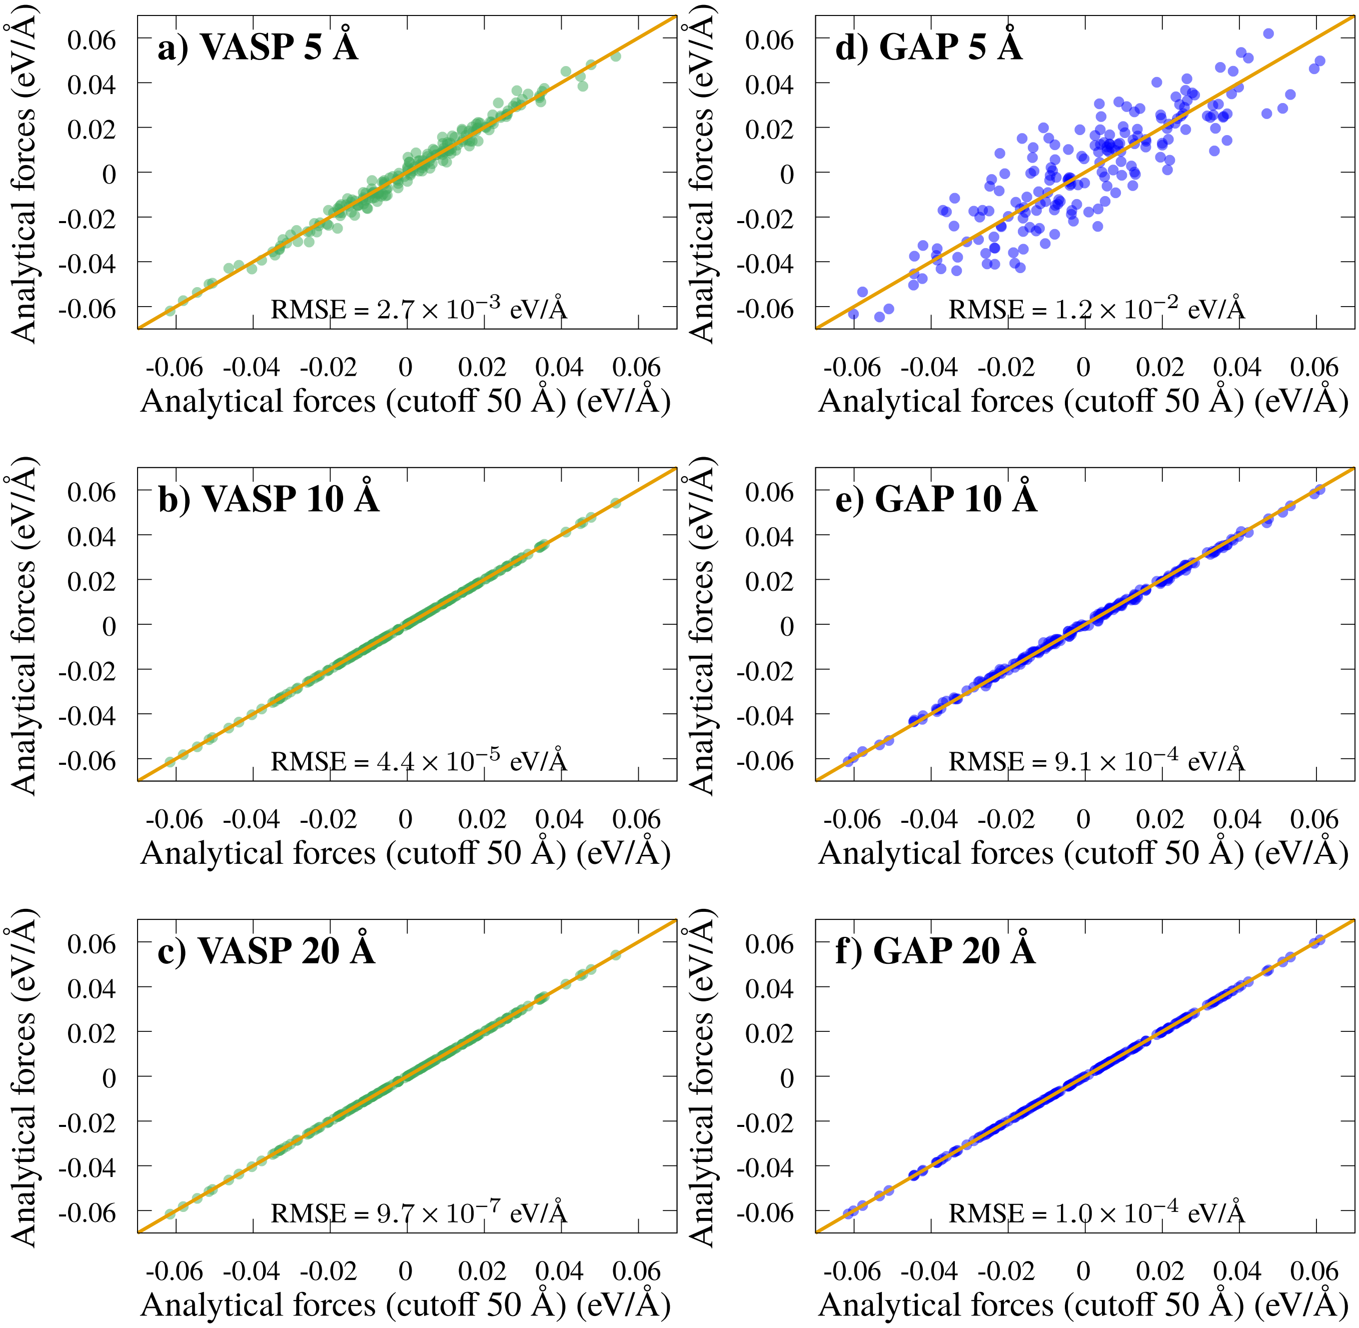


FIG. 4. Analytical dispersion forces for VASP with a) 5 Å, b) 10 Å and c) 20 Å cutoff radii compared to the VASP forces with 50 Å cutoff, and analytical dispersion forces for GAP with d) 5 Å, e) 10 Å and f) 20 Å cutoff radii compared to the GAP forces with 50 Å cutoff.

produces an additional, somewhat artificial error because the effects of the atoms in the region are damped. The region is always at the boundary of the cutoff sphere and changes based on the chosen cutoff. If the buffer region and the gradients are neglected, the errors of the GAP dispersion forces are practically identical to those of VASP forces. In Fig. 5 we show the effect of the chosen vdW cutoff on the PES of the low-temperature $C_{60}$ crystal structure as a function of rotation angle (top) and lattice parameter (bottom). The PES converges quickly with respect to the vdW cutoff, and at and above 15 Å the change in cohesive energy per atom is below 1 meV. The results shown in both Fig. 4 and Fig. 5 justify our choice of vdW cutoff for the $C_{60}$ simulations (20 Å).

[1] G. Kresse and J. Furthmüller, "Efficient iterative schemes for ab initio total-energy calculations using a plane-wave basis set," Phys. Rev. B **54**, 11169–11186 (1996).

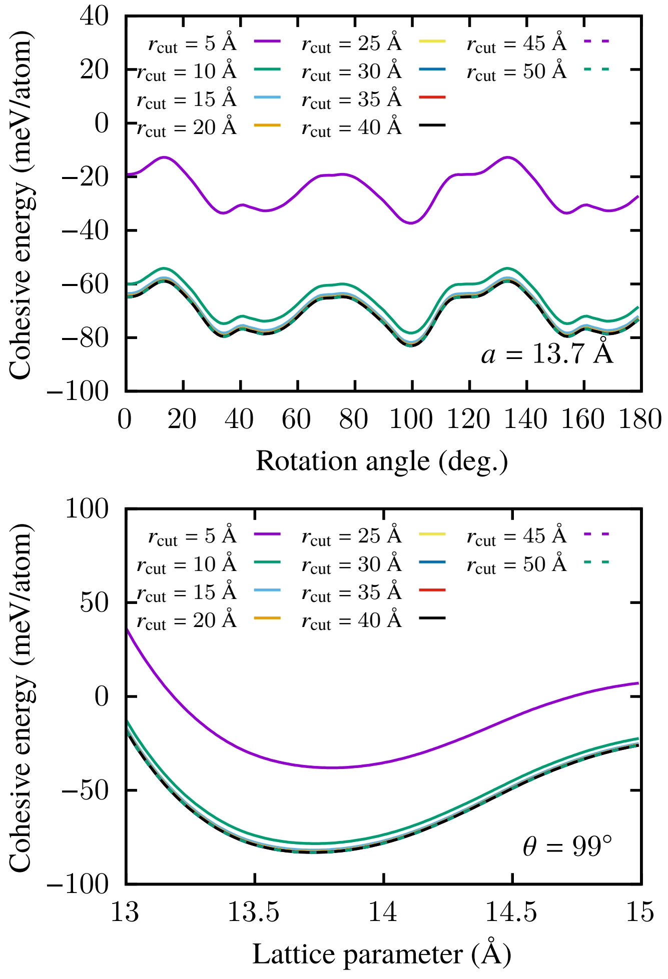


FIG. 5. Potential energy surface of the simple-cubic low-temperature $C_{60}$ crystal lattice as a function of (top) rotation angle of the $C_{60}$ units (see manuscript for details) and (bottom) lattice parameter, for different choices of vdW cutoff.


[2] G. Kresse and D. Joubert, "From ultrasoft pseudopotentials to the projector augmented-wave method," Phys. Rev. B **59**, 1758–1775 (1999).

[3] J. P. Perdew, K. Burke, and M. Ernzerhof, "Generalized gradient approximation made simple," Phys. Rev. Lett. **77**, 3865 (1996).

[4] A. Tkatchenko and M. Scheffler, "Accurate molecular van der Waals interactions from ground-state electron density and free-atom reference data," Phys. Rev. Lett. **102**, 073005 (2009).

[5] A. P. Bartók and G. Csányi, "Gaussian approximation potentials: A brief tutorial introduction," International Journal of Quantum Chemistry **115**, 1051–1057 (2015).

[6] M. A. Caro, "Optimizing many-body atomic descriptors for enhanced computational performance of machine learning based interatomic potentials," Phys. Rev. B **100**, 024112 (2019).

[7] P. Jurečka, J. Černỳ, P. Hobza, and D. R. Salahub, "Density functional theory augmented with an empirical dispersion term. interaction energies and geometries of 80 noncovalent complexes compared with ab initio quantum mechanics calculations," J. Comput. Chem. **28**, 555 (2007).

[8] N. Marom, A. Tkatchenko, M. Rossi, V. V. Gobre, O. Hod, M. Scheffler, and L. Kronik, "Dispersion interactions with density-functional theory: benchmarking semiempirical and interatomic pairwise corrected density functionals," J. Chem. Theory Comput. **7**, 3944 (2011).

[9] M. A. Caro, "Parametrization of the Tkatchenko-Scheffler dispersion correction scheme for popular exchange-correlation density functionals," arXiv:1704.00761 (2017).

[10] A. Tkatchenko, R. A. DiStasio Jr, R. Car, and M. Scheffler, "Accurate and efficient method for many-body van der Waals interactions," Phys. Rev. Lett. **108**, 236402 (2012).

[11] T. Bučko, S. Lebègue, T. Gould, and J. G. Ángyán, "Many-body dispersion corrections for periodic systems: an efficient reciprocal space implementation," J. Phys.: Condens. Matter **28**, 045201 (2016).

[12] A. Larsen, J. Mortensen, J. Blomqvist, I. Castelli, R. Christensen, M. Dulak, J. Friis, M. Groves, B. Hammer, C. Hargus, E. Hermes, P. Jennings, P. Jensen, J. Kermode, J. Kitchin, E. Kolsbjerg, J. Kubal, K. Kaasbjerg, S. Lysgaard, J. Maronsson, T. Maxson, T. Olsen, L. Pastewka, A. Peterson, C. Rostgaard, J. Schiøtz, O. Schütt, M. Strange, K. Thygesen, T. Vegge, L. Vilhelmsen, M. Walter, Z. Zeng, and K. W. Jacobsen, "The Atomic Simulation Environment – A Python library for working with atoms," J. Phys.: Condens. Matter **29**, 273002 (2017).

[13] V. L. Deringer and G. Csányi, "Machine learning based interatomic potential for amorphous carbon," Phys. Rev. B **95**, 094203 (2017).
